# Supplementary material for: Coupling of magnetism and transport properties to the lattice degrees of freedom in NdBaCo$_2$O$_{5+{\delta}}$ ($\delta \sim 0.65$)
Source: arXiv:2408.02974 source file (2024-08-06)
Supplement: Supplementary file 1 [file Supplementary_Material.pdf]

# Supplementary Material

## Coupling of magnetism and transport properties to the lattice degrees of freedom in $NdBaCo_2O_{5+\delta}$ ($\delta = 0.65$)

Himanshu Pant[1] Saurabh Singh[2,3], Jaskirat Brar[1], Priyamedha Sharma[1], M. Bharath[1], Kentaro Kuga[2], Tsunehiro Takeuchi[2,3], and R. Bindu[1*]

[1] School of Physical Sciences, Indian Institute of Technology Mandi - Kamand, Himachal Pradesh-175005, India.

[2]Toyota Technological Institute, Nagoya, Aichi 468-8511, Japan and

[3]Japan Science and Technology Agency, Kawaguchi, Saitama 332-0012, Japan

[*]bindu@iitmandi.ac.in

Contents:

a) Structural characterization for sample 2
b) Magnetic characterization for sample 2

## Structural characterization for sample 2

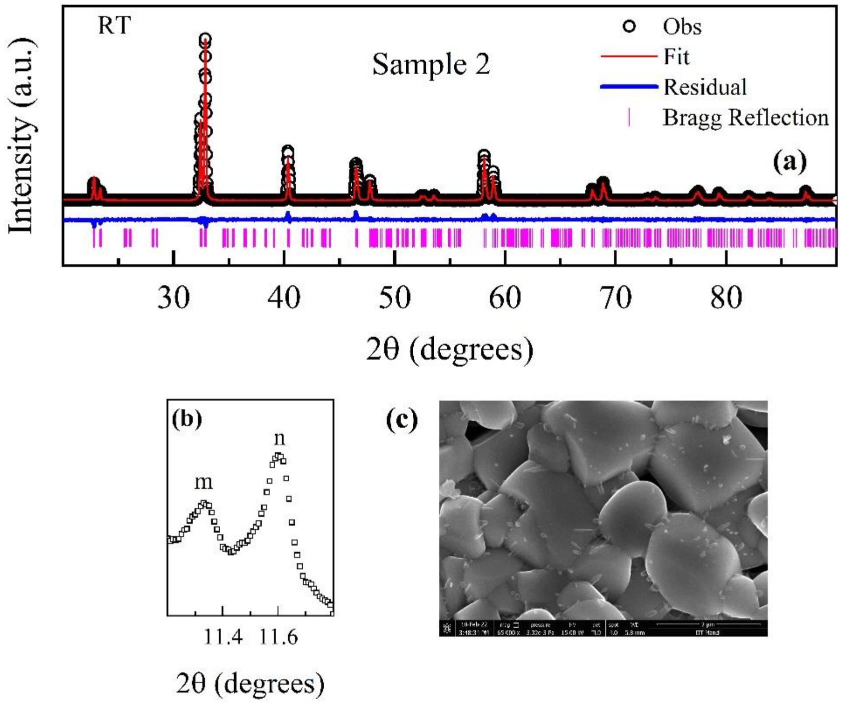


Figure S1 – For sample 2, (a) Rietveld refinement of xrd pattern collected at RT (300 K); (b) the characteristic peaks for oxygen vacancy ordering at RT; (c) SEM image.

## Magnetic characterization for sample 2

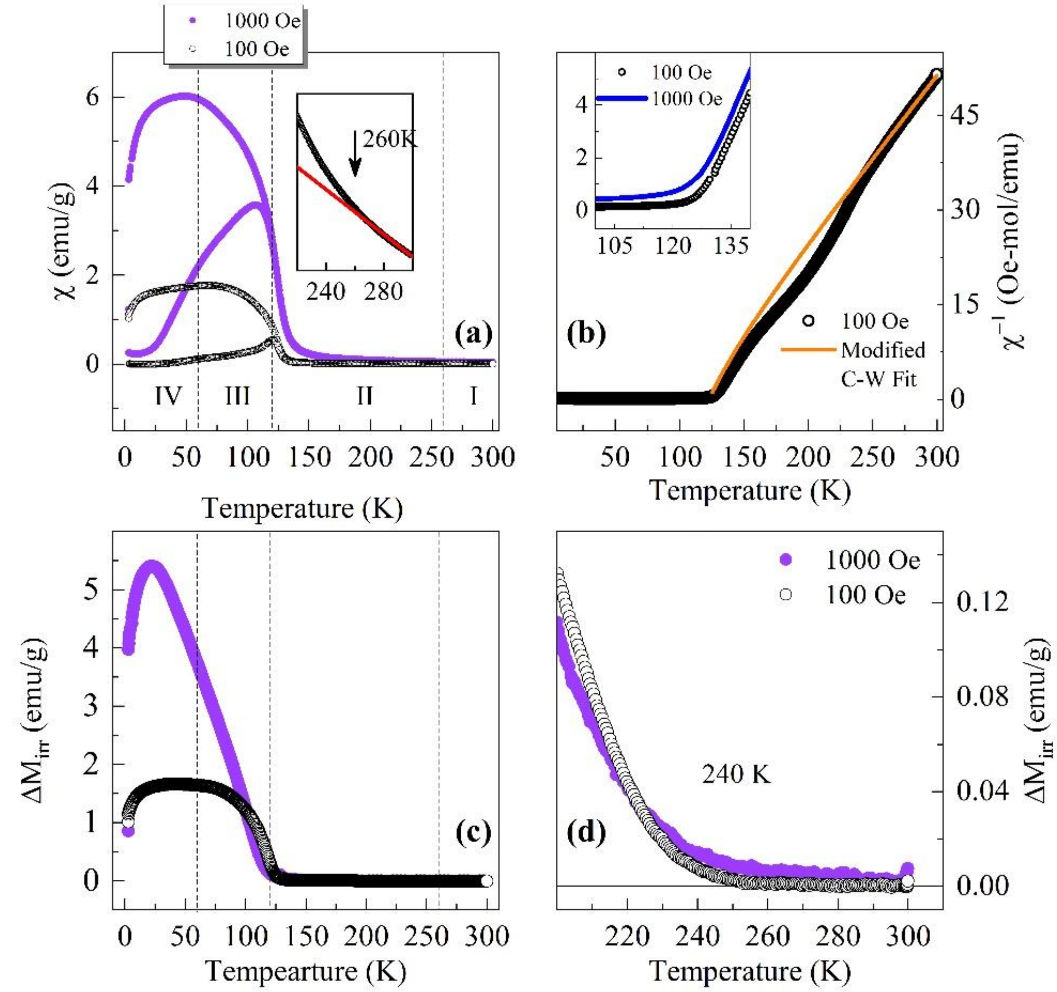


Figure S2– For sample 2, temperature dependent (a) dc susceptibility at applied magnetic field of 100 Oe and 1000 Oe during ZFC and FC; inset plot in the temperature range 220 to 300 K for ZFC at 100 Oe. (b) inverse molar susceptibility at 100 Oe during FC and extrapolated modified C-W fit till $T_c$, inset shows the inverse molar susceptibility at an applied field of 100 and 1000 Oe in FC in temperature range 100 K – 140 K; (c) and (d) $\Delta M_{irr}$ i.e. $M_{ZFC}$-$M_{FC}$, in different temperature ranges.
